# Supplementary material for: Stability-Guaranteed Reinforcement Learning for Contact-rich Manipulation
Source: arXiv:2004.10886 source file (2020-09-27)
Supplement: Supplementary file 1 [file appendix.tex]

\section{APPENDIX}\label{sec:app}

% The Wishart distribution has the following details \cite{bishop:2006:PRML}:
% \begin{align}
%     \mathcal{W}_D(S|\nu,W) &= \frac{1}{Z_W}|S|^{(\nu-D-1)/2}\exp\left(-\frac{1}{2}\textbf{Tr}(W^{-1}S)\right)\label{eqn:wishart_density}\\
%     Z_W &= 2^{\nu D/2}\Gamma_D(\nu/2)|W|^{\nu/2}\nonumber\\
%     \Gamma_D(\nu/2) &= \prod_{i=1}^D\Gamma\left(\frac{\nu+1-i}{2}\right)\nonumber\\
%     H[S] &= \ln~Z_W-\frac{\nu-D-1}{2}\mathbb{E}[\ln~|S|]+\frac{\nu D}{2}\label{eqn:wishart_entropy}\\
%     \mathbb{E}[\ln~|S|] &= \sum_{i=1}^D\psi\left(\frac{\nu+1-i}{2}\right)+D~\ln~2+\ln~|W|\nonumber
% \end{align}
% The same notations introduced in Sec. \ref{sec:background_wishart} applies. $\Gamma$ and $\psi$ are the Gamma and digamma functions, respectively.
